# Supplementary material for: Toward Enhanced Inertial Sensing via Dynamically Soft Topological States in Piezoelectric Microacoustic Metamaterials
Source: arXiv:2512.04382 source file (2025-12-04)
Supplement: Supplementary file 1 [file SupportingInformation_ArXiV.pdf]

# Supporting Information

**Toward Enhanced Inertial Sensing via Dynamically Soft Topological States in Piezoelectric Microacoustic Metamaterials**

*Onurcan Kaya, Niccolò Scalise Pantuso, Marco Galli, Jacopo M. De Ponti, Tommaso Maggioli, Davide Pavesi, Siddhartha Ghosh, Attilio Frangi, Luca Colombo, Benyamin Davaji, Matteo Rinaldi, David Horsley, Cristian Cassella****

**List of acronyms and symbols**

| Acronym/Symbol | Definition |
|---|---|
| $a$ | Pitch of the unit cell |
| **A** | A stiffness matrix in toy model, whose elements characterize the motion of $m_A$, corresponding the propagation of antisymmetric modes when they are completely uncoupled |
| $A_{k,l}$ | An element of **A** located at $k^{th}$ row and $l^{th}$ column |
| Al | Aluminum |
| AlScN | Aluminum Scandium Nitride |
| BAW | Bulk acoustic wave |
| BS | Beam splitter |
| **C** | A stiffness matrix in toy model, which introduces coupling between symmetric and antisymmetric waves |
| $C_{k,l}$ | An element of **C** located at $k^{th}$ row and $l^{th}$ column |
| $C_{Local}$ | Local dynamic compliance |
| $C_{modal}$ | Modal compliance |
| Coupled-AS | Coupled antisymmetric symmetric |
| CVRG | Capacitive vibratory rate gyroscope |
| $\delta$ | Spacing between rods |
| $\Delta T$ | Local Temperature Change |
| DUT | Device under test |
| F | Force |
| $f_{IS-1}$ | Frequency of IS-1 |
| FEM | Finite element methods |
| $\eta$ | Damping ratio |
| HF | Hydrofluoric acid |
| ICP | Inductively Coupled Plasma |
| IS | Interface State |
| IS-1 | The first interface state |
| IS-2 | The second interface state |
| K | Stiffness matrix |
| $K_{k,l}$ | An element of **K** located at $k^{th}$ row and $l^{th}$ column |
| $k_1$ | Intra-cell/inter-cell spring coefficient between lumped masses $m_A$ |
| $k_2$ | Inter-cell/intra-cell spring coefficient between lumped masses $m_A$ |
| $k_3$ | Intra-cell/inter-cell spring coefficient between lumped masses $m_S$ |
| $k_4$ | Inter-cell/intra-cell spring coefficient between lumped masses $m_S$ |
| $\kappa$ | Wavevector |
| $KE_{tot}$ | Total kinetic energy |
| $k_{eff}$ | Effective stiffness |
| $l$ | Length of the Rayleigh structure |

**List of symbols and acronyms (cont'd)**

| Acronym/Symbol | Definition |
|---|---|
| LDV | Laser Doppler vibrometer |
| **M** | Mass matrix |
| $m_{eff}$ | Effective mass |
| $m$ | Mass index |
| $m_i$ | Normalized mass index |
| $m_A$ | A lumped mass in the toy model capturing propagation of antisymmetric modes of vibration |
| MEMS | Microelectromechanical systems |
| $m_S$ | A lumped mass in the toy model capturing propagation of symmetric modes of vibration |
| $n$ | Cell index |
| $\omega$ | Angular frequency |
| $\omega_d$ | Angular excitation frequency |
| $\omega_k$ | Eigenvalue |
| $\omega_{res}$ | Angular resonance frequency |
| $p$ | Number of lumped masses per row in the supercell of the topological structure |
| P | Parity |
| PBS | Polarized beam splitter |
| PC | Periodic chain |
| PC* | Inverted periodic chain |
| PCB | Printed Circuit board |
| PD | Photodiode |
| PECVD | Plasma enhanced chemical vapor deposition |
| $\phi_k$ | Mass normalized eigenvector |
| PID | Proportional integral derivative |
| *PMG* | Piezoelectric microacoustic gyroscope |
| PS | Periodic structure |
| Pt | Platinum |
| $P_{abs}$ | Absorbed power by the device |
| $P_{in}$ | Input power to the device |
| $P_{out}$ | Output power from the device |
| $q$ | Wavenumber |
| Q | Quality factor |
| $Q_{3\text{-dB}}$ | 3-dB quality factor |
| $r$ | Number of lumped masses in the uncoupled-A structure |
| RF | Radio frequency |
| RIE | Reactive Ion Etching |

**List of symbols and acronyms (cont'd)**

| Acronym/Symbol | Definition |
|---|---|
| $s$ | Spring constant for the coupling springs between $m_A$ and $m_S$ |
| **S** | A stiffness matrix in toy model, whose elements characterize the motion of $m_S$, corresponding the propagation of symmetric modes when they are completely uncoupled. |
| $S_{k,l}$ | An element of **S** located at $k^{th}$ row and $l^{th}$ column |
| S2P | 2-Port scattering |
| SAW | Surface acoustic wave |
| SEM | Scanning electron microscopy |
| Si | Silicon |
| $SiO_2$ | Silicon oxide |
| SSH | Su-Schrieffer-Heeger |
| $t$ | Number of lumped masses in the uncoupled-S structure |
| $t_{Al}$ | Thickness of the aluminum electrodes |
| $t_{AlScN}$ | Thickness of the aluminum scandium nitride layer |
| TCE | Temperature coefficient of elastic modulus |
| $\theta_{zak}$ | Zak phase |
| $t_{Pt}$ | Thickness of the platinum layer |
| $t_{SiO2}$ | Thickness of the $SiO_2$ rods |
| $u_i^{(n)}$ | Displacement of $i^{th}$ $m_A$ in $n^{th}$ cell of the toy model |
| $UC_A$ | Unit cell of the uncoupled-A structure |
| $UC_C$ | Unit cell of the coupled-AS structure |
| $UC_C^*$ | Inverted $UC_C$ |
| $UC_S$ | Unit cell of the uncoupled-S structure |
| $UC_1$ | Unit cell-1 of the reported topological device |
| $UC_1^u$ | $UC_1$ with uniform rod distribution |
| $UC_2$ | Unit cell-2 of the reported topological device |
| $UC_2^u$ | $UC_2$ with uniform rod distribution |
| Uncoupled-A | Uncoupled antisymmetric |
| Uncoupled-S | Uncoupled symmetric |
| $v_i^{(n)}$ | Displacement of $i^{th}$ $m_S$ in $n^{th}$ cell of the toy model |
| $v_{max}$ | The maximum particle velocity |
| VNA | Vector network analyzer |
| $w_{el}$ | Width of an aluminum electrode |
| $w_{Rod}$ | Width of a rod |
| **x** | Displacement vector |
| $XeF_2$ | Xenon difluoride |
| $y$ | Number of lumped masses per row in the topological structure |

## S1. Geometrical Parameters of the Topological Device

As described in the main manuscript, the topological device consists of two different unit cell structures, as shown in Figure 1c of the main manuscript. Geometric parameters of these unit cells are listed in Figure S1, and their corresponding values are listed in Table S1 below.

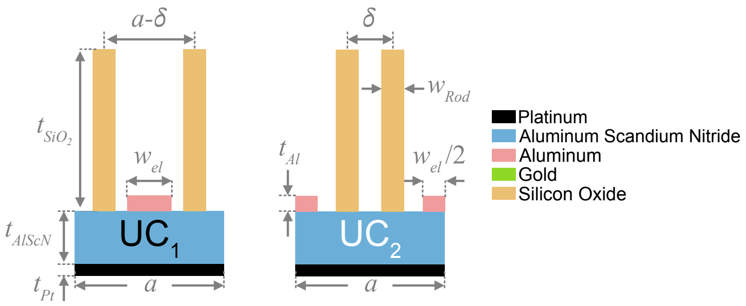


Figure S1: Geometric parameters of unit cell-1 ($UC_1$) and unit cell-2 ($UC_2$)

**Table S1 List of geometric parameters of UC1 and $UC_2$**

| Parameter | Definition | Value |
|---|---|---|
| $a$ | Pitch of the unit cell | 24 µm |
| $\delta$ | Spacing between rods for $UC_2$ | 7 µm |
| $t_{Pt}$ | Thickness of the platinum layer | 90 nm |
| $t_{AlScN}$ | Thickness of the aluminum scandium nitride layer | 500 nm |
| $t_{SiO2}$ | Thickness of the silicon dioxide rods | 1.9 µm |
| $t_{Al}$ | Thickness of the aluminum electrodes | 150 nm |
| $w_{Rod}$ | Width of a rod | 3 µm |
| $w_{el}$ | Width of an aluminum electrode | 6 µm |

## S2. Toy Model Dispersion Analysis

This section describes the derivation of the dispersion curves for the toy models relative to the two uncoupled structures named uncoupled antisymmetric (uncoupled-A) and uncoupled symmetric (uncoupled-S) structures (Figure S2a), the coupled antisymmetric symmetric structure named coupled-AS structure (Figure S2b) and the topological structure (Figure S2c). For each structure, the displacements of the red masses in the top row (representing the propagation of antisymmetric waves) and of the black masses in the bottom row (representing the propagation of symmetric waves) are denoted by $u_m^{(n)}$ and $v_m^{(n)}$, respectively, where the subscript $m$ indicates the mass index within a given cell and the superscript $n$ is the cell index. The parameter values used in these dispersion analyses are listed in Table S2. The next three subsections present the derivation of the eigenvalue problems for each structure, and the last subsection outlines the procedure used to obtain the corresponding dispersion curves.

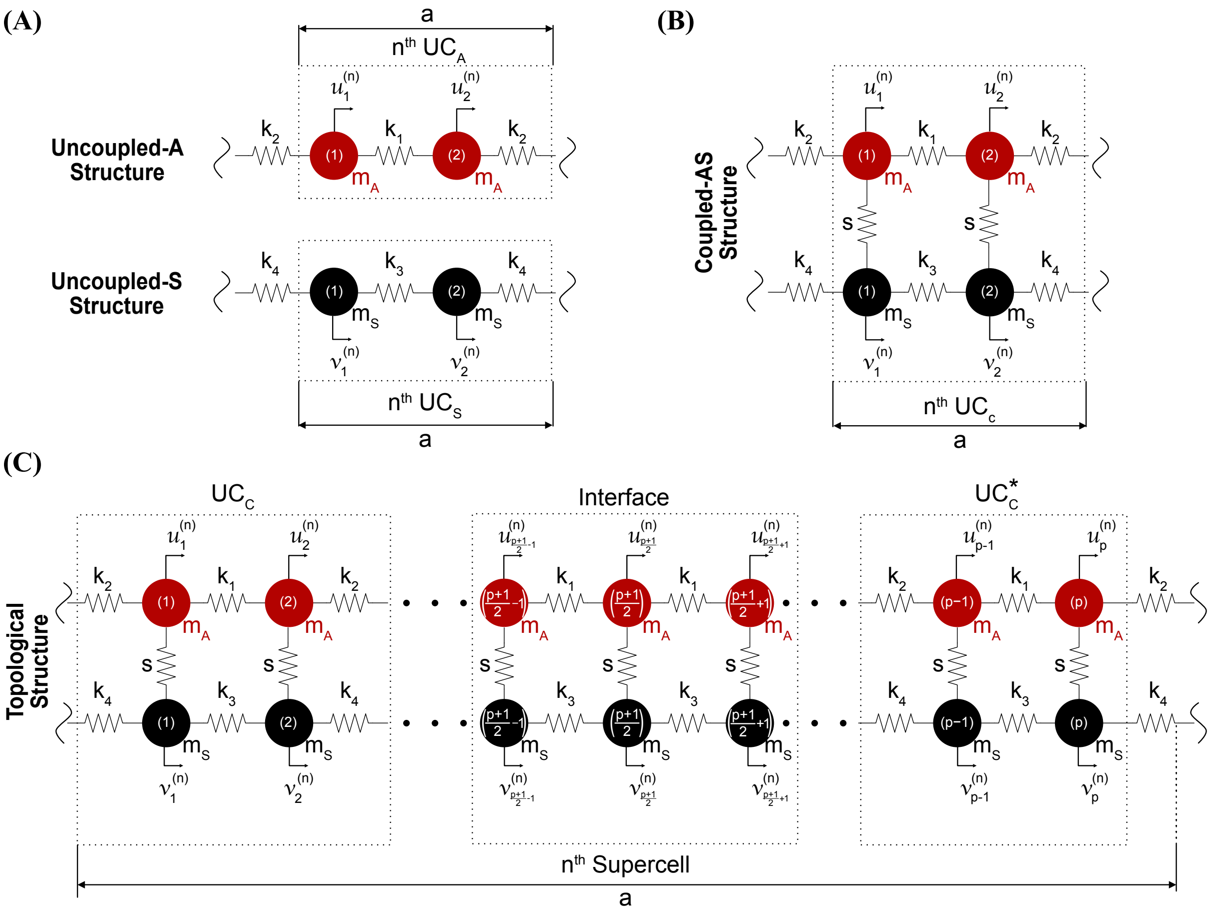


Figure S2: Geometries considered during the dispersion analyses for the toy models presented in Figure 2 of main manuscript: (a) unit cells of the uncoupled-antisymmetric (uncoupled-A) and uncoupled-symmetric (uncoupled-S) structures; (b) unit cell of the coupled antisymmetric-symmetric (coupled-AS) structure; and (c) supercell for the topological structure.

**Table S2 List of parameters used in dispersion analysis**

| Parameter | Definition | Value |
|---|---|---|
| $m_A$ | Mass of a lumped mass capturing propagation of antisymmetric modes of vibration | 1 |
| $m_S$ | Mass of a lumped mass capturing propagation of symmetric modes of vibration | 5 |

| | | |
|---|---|---|
| $k_1$ | Intra-cell/inter-cell spring coefficient between lumped masses $m_A$ | 1 |
| $k_2$ | Inter-cell/intra-cell spring coefficient between lumped masses $m_A$ | 1.2 |
| $k_3$ | Intra-cell/inter-cell spring coefficient between lumped masses $m_S$ | 2 |
| $k_4$ | Inter-cell/intra-cell spring coefficient between lumped masses $m_S$ | 0.8 |
| $s$ | Spring constant for the coupling springs between $m_A$ and $m_S$ | 0.5 |
| $p$ | Number of lumped masses per row in a supercell | 201 |
| $a$ | Unit cell/supercell size | 1 |

### S2.1. Uncoupled Structures

Let us write Newton's second law for each mass in the n$^{th}$ unit cell of the uncoupled-A structure described in Figure S2a. The resulting equations of motion for the first and second masses of the unit cell are given in Equations (S1.1) and (S1.2), respectively.

$$m_A \ddot{u}_1^{(n)} = k_1\left(u_2^{(n)} - u_1^{(n)}\right) - k_2\left(u_1^{(n)} - u_2^{(n-1)}\right) \tag{S1.1}$$

$$m_A \ddot{u}_2^{(n)} = k_2\left(u_1^{(n+1)} - u_2^{(n)}\right) - k_1\left(u_2^{(n)} - u_1^{(n)}\right) \tag{S1.2}$$

Assuming a plane wave solution and considering Bloch-Floquet periodic boundary conditions, the displacements of each mass can be expressed as shown in Equations (S1.3) and (S1.4).

$$u_1^{(n)} = \bar{u}_1(q)e^{i(nqa-\omega t)} \tag{S1.3}$$

$$u_2^{(n)} = \bar{u}_2(q)e^{i(nqa-\omega t)} \tag{S1.4}$$

where, $q$ is the wave number, $\omega$ is the angular frequency, $a$ is the unit cell size, and $\bar{u}_m(q)$ is the displacement amplitude of the $m^{th}$ mass. Substituting Equations (S1.3) and (S1.4) into (S1.1) and (S1.2) leads to an eigenvalue problem (see Eq. S2.5).

$$\left[\mathbf{K}(q) - \omega^2\mathbf{M}\right]\cdot\mathbf{x}(q) = 0 \tag{S1.5}$$

In Eq. S2.5, **K** is the stiffness matrix, **M** is the mass matrix, and **x** is the displacement vector. These are defined as:

$$\mathbf{K}(q) = \begin{bmatrix} k_1 + k_2 & -k_1 - k_2 e^{-iqa} \\ -k_1 - k_2 e^{iqa} & k_1 + k_2 \end{bmatrix} \tag{S1.6}$$

$$\mathbf{M} = \begin{bmatrix} m_A & 0 \\ 0 & m_A \end{bmatrix} \tag{S1.7}$$

$$\mathbf{x}(q) = \begin{bmatrix} \bar{u}_1 \\ \bar{u}_2 \end{bmatrix} \tag{S1.8}$$

The eigenvalue problem for the uncoupled-S structure can simply be obtained by replacing $k_1$ with $k_3$, $k_2$ with $k_4$, $m_A$ with $m_S$, $u_1$ with $v_1$ and, $u_2$ with $v_2$.

### S2.2. Coupled Structure

The n[th] unit cell of the coupled antisymmetric-symmetric (coupled-AS) structure is illustrated in Figure S2b. Newton's second law for the unit cell of the coupled-AS structure (UC$_c$) can be written by adding the force due to the coupling spring in the force balance equations of the uncoupled structures, i.e. equations (S1.1) and (S1.2). The resulting equations governing the motion of each mass in the top and bottom rows are given in Equations (S1.9)-(S1.10) and (S1.11)-(S1.12), respectively.

$$m_A\ddot{u}_1^{(n)} = k_1\left(u_2^{(n)} - u_1^{(n)}\right) - k_2\left(u_1^{(n)} - u_2^{(n-1)}\right) - s\left(u_1^{(n)} - v_1^{(n)}\right) \quad \text{(S1.9)}$$

$$m_A\ddot{u}_2^{(n)} = k_2\left(u_1^{(n+1)} - u_2^{(n)}\right) - k_1\left(u_2^{(n)} - u_1^{(n)}\right) - s\left(u_2^{(n)} - v_2^{(n)}\right) \quad \text{(S1.10)}$$

$$m_S\ddot{v}_1^{(n)} = k_3\left(v_2^{(n)} - v_1^{(n)}\right) - k_4\left(v_1^{(n)} - v_2^{(n-1)}\right) - s\left(v_1^{(n)} - u_1^{(n)}\right) \quad \text{(S1.11)}$$

$$m_S\ddot{v}_2^{(n)} = k_4\left(v_1^{(n+1)} - v_2^{(n)}\right) - k_3\left(v_2^{(n)} - v_1^{(n)}\right) - s\left(v_2^{(n)} - u_2^{(n)}\right) \quad \text{(S1.12)}$$

Similarly, assuming a plane wave solution and Bloch-Floquet periodic boundary conditions

$$u_m^{(n)} = \tilde{u}_i(q)e^{i(nqa-\omega t)}, \quad m=1,2 \quad \text{(S1.13)}$$

$$v_m^{(n)} = \tilde{v}_m(q)e^{i(nqa-\omega t)}, \quad m=1,2 \quad \text{(S1.14)}$$

where $\tilde{u}_m^n(q)$ and $\tilde{v}_m^n(q)$ are the displacement amplitudes of the corresponding masses in top and bottom rows respectively. Similarly, substituting Equations (S1.13) and (S1.14) into Equations (S1.9)–(S1.12) gives the eigenvalue problem:

$$\left[\mathbf{K}(q) - \omega^2\mathbf{M}\right]\cdot\mathbf{x}(q) = 0 \quad \text{(S1.15)}$$

where, the stiffness matrix (**K**), the mass matrix (**M**), and the displacement vector (**x**) are defined as shown in Equations (S1.16), (S1.17), and (S1.18), respectively.

$$\mathbf{K}(q) = \begin{bmatrix} k_1+k_2+s & -k_1-k_2e^{-iqa} & -s & 0 \\ -k_1-k_2e^{iqa} & k_1+k_2+s & 0 & -s \\ -s & 0 & k_3+k_4+s & -k_3-k_4e^{-iqa} \\ 0 & -s & -k_3-k_4e^{iqa} & k_3+k_4+s \end{bmatrix} \quad \text{(S1.16)}$$

$$\mathbf{M} = \begin{bmatrix} m_A & 0 & 0 & 0 \\ 0 & m_A & 0 & 0 \\ 0 & 0 & m_S & 0 \\ 0 & 0 & 0 & m_S \end{bmatrix} \quad \text{(S1.17)}$$

$$\mathbf{x}(q)=\begin{bmatrix}\bar{u}_1\\ \bar{u}_2\\ \bar{v}_1\\ \bar{v}_2\end{bmatrix} \tag{S1.18}$$

### S2.3. Topological Structure

The toy model employed for the supercell dispersion analysis of the topological structure is given in Figure S2c. Both the top and the bottom rows within the supercell consist of a number $p$ of masses. As described in the main manuscript, the topological structure consists of two periodic chains (PCs), namely PC and PC$^*$. PC and PC$^*$ are formed by repeating $UC_c$ and $UC_c^*$ by (p-1)/2 times, respectively. Then, PC and PC$^*$ are combined through a common interface forming the topological structure. Assuming Bloch-Floquet periodic boundary conditions, the eigenvalue problem derivation for the supercell dispersion analysis is presented below.

Firstly, let us write the Newton's second law for: (i) the first mass pair in the n$^{th}$ supercell– specifically, the first mass in the top row [Equation (S1.19)] and in the bottom row [Equation (S1.20)]–

$$m_A\ddot{u}_1^{(n)}=k_1\left(u_2^{(n)}-u_1^{(n)}\right)-k_2\left(u_1^{(n)}-u_p^{(n-1)}\right)-s\left(u_1^{(n)}-v_1^{(n)}\right) \tag{S1.19}$$

$$m_S\ddot{v}_1^{(n)}=k_3\left(v_2^{(n)}-v_1^{(n)}\right)-k_4\left(v_1^{(n)}-v_p^{(n-1)}\right)-s\left(v_1^{(n)}-u_1^{(n)}\right) \tag{S1.20}$$

(ii) the last mass pair in the n$^{th}$ supercell– specifically, the last mass in the top row [Equation (S1.21)] and in the bottom row [Equation (S1.22)]–,

$$m_A\ddot{u}_p^{(n)}=k_2\left(u_1^{(n+1)}-u_p^{(n)}\right)-k_1\left(u_p^{(n)}-u_{p-1}^{(n)}\right)-s\left(u_p^{(n)}-v_p^{(n)}\right) \tag{S1.21}$$

$$m_S\ddot{v}_p^{(n)}=k_4\left(v_1^{(n+1)}-v_p^{(n)}\right)-k_3\left(v_p^{(n)}-v_{p-1}^{(n)}\right)-s\left(v_p^{(n)}-u_p^{(n)}\right) \tag{S1.22}$$

(iii) for the remaining masses in the top row–specifically, the masses in PC [Equation (S1.23) ], the mass at the interface [Equation (S1.24)] , and the masses in PC$^*$ [Equation (S1.25)]–and

$$m_A\ddot{u}_m^{(n)}=k_2\left(u_{m+1}^{(n)}-u_m^{(n)}\right)-k_1\left(u_m^{(n)}-u_{m-1}^{(n)}\right)-s\left(u_m^{(n)}-v_m^{(n)}\right)\quad \text{for}\quad m\in\mathbb{Z}\cap\left[2,\frac{p+1}{2}\right) \tag{S1.23}$$

$$m_A\ddot{u}_m^{(n)}=k_1\left(u_{m+1}^{(n)}-u_m^{(n)}\right)-k_1\left(u_m^{(n)}-u_{m-1}^{(n)}\right)-s\left(u_m^{(n)}-v_m^{(n)}\right)\quad \text{for}\quad m=\frac{p+1}{2} \tag{S1.24}$$

$$m_A\ddot{u}_m^{(n)}=k_1\left(u_{m+1}^{(n)}-u_m^{(n)}\right)-k_2\left(u_m^{(n)}-u_{m-1}^{(n)}\right)-s\left(u_m^{(n)}-v_m^{(n)}\right)\quad \text{for}\quad m\in\mathbb{Z}\cap\left(\frac{p+1}{2},p\right) \tag{S1.25}$$

(iv) for the remaining masses in the bottom row–specifically, the masses in PC [Equation (S1.26)], the mass at the interface [Equation (S1.27)] , and the masses in PC$^*$ [Equation (S1.28)]–

$$m_S\ddot{v}_i^{(n)}=k_4\left(v_{m+1}^{(n)}-v_m^{(n)}\right)-k_3\left(v_m^{(n)}-v_{m-1}^{(n)}\right)-s\left(v_m^{(n)}-u_m^{(n)}\right)\quad \text{for}\quad m\in\mathbb{Z}\cap\left[2,\frac{p+1}{2}\right) \tag{S1.26}$$

$$m_S \ddot{v}_m^{(n)} = k_3\left(v_{m+1}^{(n)} - v_m^{(n)}\right) - k_3\left(v_m^{(n)} - v_{m-1}^{(n)}\right) - s\left(v_m^{(n)} - u_m^{(n)}\right) \quad \text{for} \quad m = \frac{p+1}{2} \tag{S1.27}$$

$$m_S \ddot{v}_m^{(n)} = k_3\left(v_{m+1}^{(n)} - v_m^{(n)}\right) - k_4\left(v_m^{(n)} - v_{m-1}^{(n)}\right) - s\left(v_m^{(n)} - u_m^{(n)}\right) \quad \text{for} \quad m \in \mathbb{Z} \cap \left(\frac{p+1}{2}, p\right) \tag{S1.28}$$

Assuming a plane wave solution and applying Bloch-Floquet periodic boundary conditions, the displacement relation between the $n^{\text{th}}$ supercell and its adjacent *(n-1)*$^{\text{th}}$ and *(n+1)*$^{\text{th}}$ supercells can be expressed as shown in Equations (S1.29)-(S1.30) and (S1.31)-(S1.32), respectively.

$$u_p^{(n-1)} = u_p^{(n)}(q)e^{-iqa} \tag{S1.29}$$

$$v_p^{(n-1)} = v_p^{(n)}(q)e^{-iqa} \tag{S1.30}$$

$$u_1^{(n+1)} = u_1^{(n)}(q)e^{iqa} \tag{S1.31}$$

$$v_1^{(n+1)} = v_1^{(n)}(q)e^{iqa} \tag{S1.32}$$

Substituting Equations (S1.29)–(S1.32) into Equations (S1.19)–(S1.28) and rearranging gives the eigenvalue problem in Equation (S1.33).

$$\left[\mathbf{K}(q) - \omega^2 \mathbf{M}\right] \cdot \mathbf{x}(q) = 0 \tag{S1.33}$$

where, **K** and **M** are *2p* × *2p* square matrices and **x** is a column vector with size *2p*. **M** is a diagonal matrix, as shown in equation (S1.34). Its first *p* diagonal elements correspond to the masses in the top row, which characterizes the propagation of antisymmetric waves and are all equal to $m_A$, while its last *p* diagonal elements represent the masses in the bottom row, which characterize the propagation of symmetric waves and are all equal to $m_S$.

$$\mathbf{M} = \begin{bmatrix} \begin{bmatrix} m_A & \cdots & 0 \\ \vdots & \ddots & \vdots \\ 0 & \cdots & m_A \end{bmatrix}_{\text{p x p}} & \boxed{0}_{\text{p x p}} \\ \boxed{0}_{\text{p x p}} & \begin{bmatrix} m_S & \cdots & 0 \\ \vdots & \ddots & \vdots \\ 0 & \cdots & m_S \end{bmatrix}_{\text{p x p}} \end{bmatrix} \tag{S1.34}$$

The matrix **K** is constructed by combining four *p* × *p* square matrices, denoted by **A**, **S**, and **C,** as shown in equation (S1.35). The elements of matrices **A** and **S** characterize the motion of the masses along the top and bottom rows, respectively, corresponding to the propagation of antisymmetric and symmetric waves when they are completely uncoupled. The coupling between the antisymmetric and symmetric waves is introduced through the matrix **C**.

$$\mathbf{K}=\begin{bmatrix} \boxed{\begin{matrix} A_{1,1} & A_{1,2} & 0 & A_{1,p} \\ A_{2,1} & A_{2,2} & \ddots & 0 \\ 0 & \ddots & \ddots & A_{p-1,p} \\ A_{p,1} & 0 & A_{p,p-1} & A_{p,p} \end{matrix}} & \boxed{\begin{matrix} C_{1,1} & 0 & 0 & 0 \\ 0 & C_{2,2} & 0 & 0 \\ 0 & 0 & \ddots & 0 \\ 0 & 0 & 0 & C_{p,p} \end{matrix}} \\ \boxed{\begin{matrix} C_{1,1} & 0 & 0 & 0 \\ 0 & C_{2,2} & 0 & 0 \\ 0 & 0 & \ddots & 0 \\ 0 & 0 & 0 & C_{p,p} \end{matrix}} & \boxed{\begin{matrix} S_{1,1} & S_{1,2} & 0 & S_{1,p} \\ S_{2,1} & S_{2,2} & \ddots & 0 \\ 0 & \ddots & \ddots & S_{p-1,p} \\ S_{p,1} & 0 & S_{p,(p-1)} & S_{p,p} \end{matrix}} \end{bmatrix} \tag{S1.35}$$

All elements of **A** and **S** are zero except for those on the main diagonal, the upper and lower diagonals, and the first and last elements of their antidiagonals. In contrast, **C** is a diagonal matrix. The specific rules governing the nonzero elements of **A**, **S**, and **C** are detailed below [see equations (S1.36), (S1.37), and (S1.38)].

$$A_{k,l}=\begin{cases} k_1+k_2 & \text{if} \quad k=l\neq\dfrac{p+1}{2} \\ 2k_1 & \text{if} \quad k=l=\dfrac{p+1}{2} \\ -\left(k_1\cdot\dfrac{1-(-1)^k}{2}+k_2\cdot\dfrac{1+(-1)^k}{2}\right) & \text{if} \quad k=l\pm1<\dfrac{p+1}{2} \\ -\left(k_1\cdot\dfrac{1+(-1)^k}{2}+k_2\cdot\dfrac{1-(-1)^k}{2}\right) & \text{if} \quad k=l\pm1\geq\dfrac{p+1}{2} \\ -k_2e^{-iqa} & \text{if} \quad k=1 \;\&\; l=p \\ -k_2e^{-iqa} & \text{if} \quad k=p \;\&\; l=1 \end{cases} \tag{S1.36}$$

$$S_{k,l}=\begin{cases} k_3+k_4 & \text{if} \quad k=l\neq\dfrac{p+1}{2} \\ 2k_3 & \text{if} \quad k=l=\dfrac{p+1}{2} \\ -\left(k_3\cdot\dfrac{1-(-1)^k}{2}+k_4\cdot\dfrac{1+(-1)^k}{2}\right) & \text{if} \quad k=l\pm1<\dfrac{p+1}{2} \\ -\left(k_3\cdot\dfrac{1+(-1)^k}{2}+k_4\cdot\dfrac{1-(-1)^k}{2}\right) & \text{if} \quad k=l\pm1\geq\dfrac{p+1}{2} \\ -k_4e^{-iqa} & \text{if} \quad k=1 \;\&\; l=p \\ -k_4e^{iqa} & \text{if} \quad k=p \;\&\; l=1 \end{cases} \tag{S1.37}$$

$$C_{k,l}=\{s \quad \text{if} \quad k=l \tag{S1.38}$$

Finally, the first $p$ elements of the column vector $\mathbf{x}$ store the displacement amplitudes of the masses in the top row, while the last $p$ elements stores those in the bottom row as, shown below in equation (S1.39).

$$\mathbf{x}(q) = \begin{bmatrix} \bar{u}_1 \\ \vdots \\ \bar{u}_p \\ \bar{v}_1 \\ \vdots \\ \bar{v}_p \end{bmatrix} \tag{S1.39}$$

**S2.4. Solving Eigenvalue Problems**

The previous sections present the eigenvalue problems for the uncoupled, coupled, and topological structures as a function of the wavenumber $q$. To obtain the dispersion curves, $q$ was swept from $-\pi/a$ to $\pi/a$, and the resulting eigenvalue problem for each $q$ value was solved numerically in MATLAB. The obtained eigenvalues were then plotted against the corresponding $q$ and are presented in Figures 2b, 2d, and 2f of the main manuscript.

## S3. Zak Phase of the Unit Cells of the Topological Structure

The topology of a one-dimensional system is characterized by the Zak phase, which is obtained by integrating the Berry connection over the first Brillouin zone [1]. In this study, the Zak phase was calculated using a discrete approach by dividing the Brillouin zone into many sufficiently small segments and by accumulation of the Berry phase as [2]:

$$e^{-i\theta_{zak}^{k}} = \prod_{j=1}^{n} \left\langle \phi_{k,j} \middle| \phi_{k,j+1} \right\rangle \tag{S2.1}$$

where, $\theta_{zak}^{k}$ is the Zak phase of k$^{\text{th}}$-band, $\phi_k$ is the corresponding eigenvector, and $n$ is the number of degrees of freedom of the system. Since both $UC_c$ and $UC_c^*$ are inversion-symmetric, their Zak phases can only be 0 (trivial) or π (nontrivial) [2]. Figure S3 reports the dispersion curves of $UC_c$ and $UC_c^*$, along with the corresponding Zak phases of each branch, confirming the Zak phase relation required for existence of the interface states.

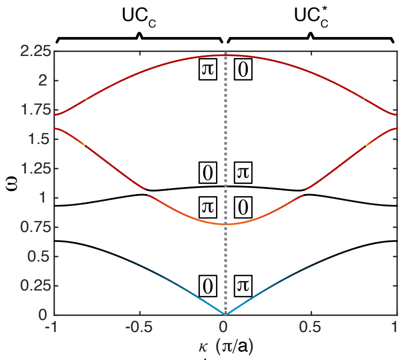


Figure S3: Dispersion curves of $UC_c$ and $UC_c^*$ along with the corresponding Zak phases for each dispersion branch.

[1] G. Li *et al.*, “Direct extraction of topological Zak phase with the synthetic dimension,” *Light Sci Appl*, vol. 12, no. 1, p. 81, Mar. 2023, doi: 10.1038/s41377-023-01126-1.

[2] H.-X. Wang, G.-Y. Guo, and J.-H. Jiang, “Band topology in classical waves: Wilson-loop approach to topological numbers and fragile topology,” *New J. Phys.*, vol. 21, no. 9, p. 093029, Sept. 2019, doi: 10.1088/1367-2630/ab3f71.

## S4. Calculation of Modal and dynamic Local Compliance for Our Toy Models

To assess the ability of interface states (ISs) to achieve higher particle velocities then trivial modes, we calculated modal compliance ($C_{modal}$) and dynamic local compliance ($C_{Local}$) for the uncoupled-A, uncoupled-S, coupled-AS, and topological structures presented in Figures 3a–3g of the main manuscript. This section outlines the details of these calculations. The employed mass-spring models for each structure are given in Figure S4. The parameter values for the mass and spring elements were identical to those listed in Table S2 for all structures, and an additional set of parameters specific to these analyses is defined in Table S4.

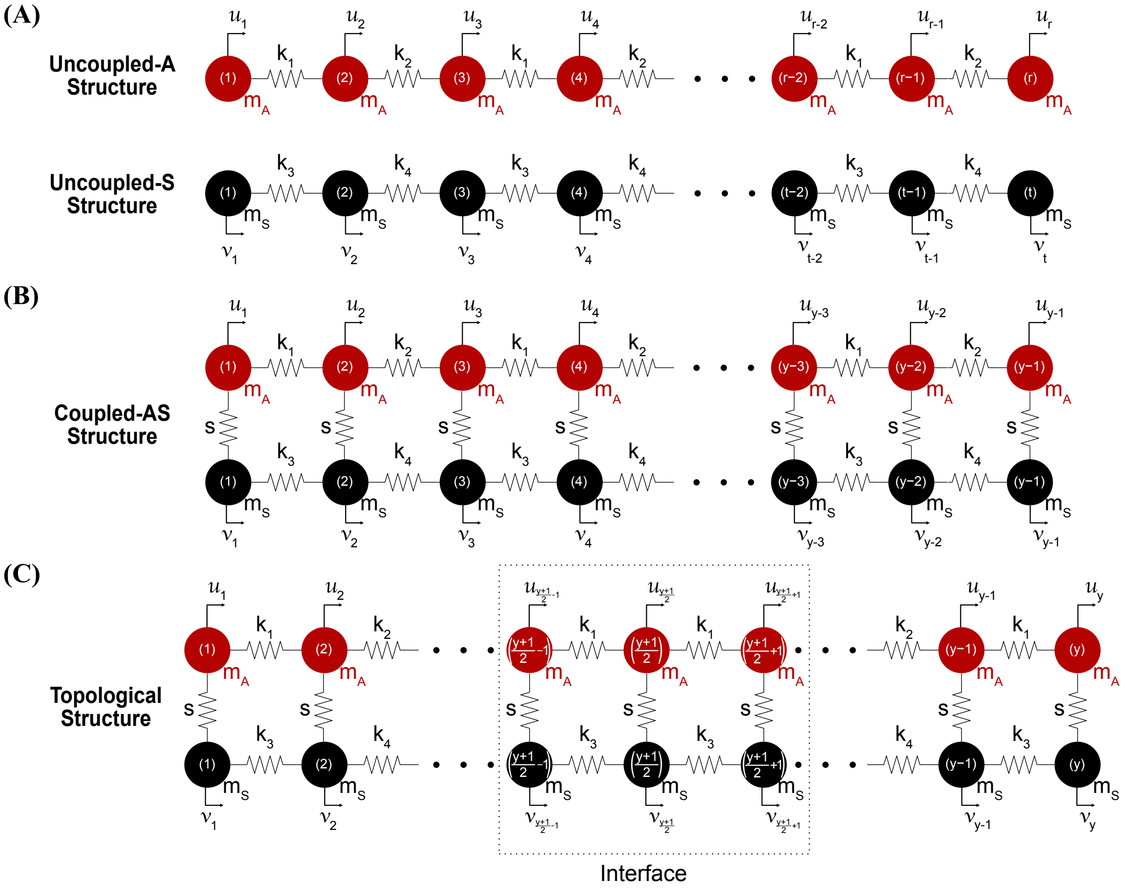


Figure S4: Employed mass-spring models for our compliance analyses: (a) uncoupled-A and uncoupled-S; (b) the coupled-AS structure; and (c) the topological structure.

**Table S4 List of additional parameters used in compliance analyses**

| Parameter | Definition | Value |
|---|---|---|
| $y$ | Number of lumped masses per row in the topological structure | 407 |
| $r$ | Number of lumped masses in the uncoupled-A structure | 2445 |
| $t$ | Number of lumped masses in the uncoupled-S structure | 489 |
| $\eta$ | Damping ratio | $10^{-4}$ |

### S4.1. Modeling the Structures

Calculating $C_{modal}$ and $C_{Local}$ requires solving the undamped free vibration problem [Equation (S4.1)] for each structure.

$$\left[\mathbf{K} - \omega^2 \mathbf{M}\right] \cdot \mathbf{x} = 0 \tag{S4.1}$$

where, **K**, **M** and **x** are stiffness, mass and displacement matrices of the corresponding structure, and they were obtained following the approach outlined in Section S2, by replacing the Bloch-Floquet periodicity with stress-free boundary conditions. The resulting **M**, **K** and ***x*** matrices for each structure are described below. The corresponding eigenvalues and mass-normalized eigenvectors for each structure were obtained numerically in MATLAB.

The uncoupled-A structure (Figure S4a) consists of *r* masses, and the corresponding **M**, **x** and **K** are obtained by eliminating equations characterizing the motion of symmetric modes and the coupling between the symmetric and antisymmetric modes from Equations (S1.19)-(S1.28) . The resulting matrices are presented below in Equations (S4.2), (S4.3) and (S4.4).

$$\mathbf{M}=\begin{bmatrix} m_A & \cdots & 0 \\ \vdots & \ddots & \vdots \\ 0 & \cdots & m_A \end{bmatrix}_{\mathrm{y\,x\,y}} \tag{S4.2}$$

$$\mathbf{x}=\begin{bmatrix} \bar{u}_1 \\ \vdots \\ \bar{u}_y \end{bmatrix} \tag{S4.3}$$

$$\mathbf{K}=\begin{bmatrix} K_{1,1} & K_{1,2} & 0 & 0 \\ K_{2,1} & K_{2,2} & \ddots & 0 \\ 0 & \ddots & \ddots & K_{y-1,y} \\ 0 & 0 & K_{y,y-1} & K_{y,y} \end{bmatrix} \tag{S4.4}$$

As shown in Equation (S4.4), replacing the Bloch-Floquet periodic boundary conditions with stress-free boundary conditions makes **K** a tri-diagonal matrix, and its non-zero elements are defined as (S4.5):

$$K_{k,l}=\begin{cases} k_1+k_2 & \text{if} \quad k=l \\ -\left(k_1\cdot\dfrac{1-(-1)^k}{2}+k_2\cdot\dfrac{1+(-1)^k}{2}\right) & \text{if} \quad k=l\pm 1 \end{cases} \tag{S4.5}$$

Related matrices for the uncoupled-S structure can be obtained by simply replacing $m_A$ with $m_S$, $k_1$ with $k_3$, $k_2$ with $k_4$ and $r$ with $t$.

The coupled structure (Figure S4b) consists of a chain of only one type of unit cell (i.e., $UC_c$). Therefore, unlike the topological structure (Figure S4c), the coupled structure does not have an interface with broken periodicity (i.e., a topological interface), as described in Section S2.3 of the Supplementary Material and Figure 2e of the main manuscript. Consequently, the coupled structure has one fewer mass in each row compared to the topological structure. As a result, the corresponding **M**, **K**, and **x** are analogous to those of the topological structure but have reduced dimensions of $(2y\text{-}2) \times (2y\text{-}2)$, $(2y\text{-}2) \times (2y\text{-}2)$, and $(2y\text{-}2) \times 1$, as shown in Equations (S4.6), (S4.7), and (S4.8), respectively.

$$\mathbf{M} = \begin{bmatrix} \boxed{\begin{matrix} m_A & \cdots & 0 \\ \vdots & \ddots & \vdots \\ 0 & \cdots & m_A \end{matrix}}_{(y\text{-}1)\times(y\text{-}1)} & \boxed{0}_{(y\text{-}1)\times(y\text{-}1)} \\ \boxed{0}_{(y\text{-}1)\times(y\text{-}1)} & \boxed{\begin{matrix} m_S & \cdots & 0 \\ \vdots & \ddots & \vdots \\ 0 & \cdots & m_S \end{matrix}}_{(y\text{-}1)\times(y\text{-}1)} \end{bmatrix} \quad \text{(S4.6)}$$

$$\mathbf{K} = \begin{bmatrix} \boxed{\begin{matrix} A_{1,1} & A_{1,2} & 0 & 0 \\ A_{2,1} & A_{2,2} & \ddots & 0 \\ 0 & \ddots & \ddots & A_{y-2,y-1} \\ 0 & 0 & A_{y-1,y-2} & A_{y-1,y-1} \end{matrix}} & \boxed{\begin{matrix} C_{1,1} & 0 & 0 & 0 \\ 0 & C_{2,2} & 0 & 0 \\ 0 & 0 & \ddots & 0 \\ 0 & 0 & 0 & C_{y-1,y-1} \end{matrix}} \\ \boxed{\begin{matrix} C_{1,1} & 0 & 0 & 0 \\ 0 & C_{2,2} & 0 & 0 \\ 0 & 0 & \ddots & 0 \\ 0 & 0 & 0 & C_{y-1,y-1} \end{matrix}} & \boxed{\begin{matrix} S_{1,1} & S_{1,2} & 0 & 0 \\ S_{2,1} & S_{2,2} & \ddots & 0 \\ 0 & \ddots & \ddots & S_{y-2,y-1} \\ 0 & 0 & S_{y,(y-1)} & S_{y-1,y-1} \end{matrix}} \end{bmatrix} \quad \text{(S4.7)}$$

$$\mathbf{x} = \begin{bmatrix} \bar{u}_1 \\ \vdots \\ \bar{u}_{y-1} \\ \bar{v}_1 \\ \vdots \\ \bar{v}_{y-1} \end{bmatrix} \quad \text{(S4.8)}$$

As we did in section S2.3, **K** can be decomposed into four *(y-1)* × *(y-1)* square matrices, namely **A**, **S,** and **C**, as shown in Equation(S4.7). Evidently, replacing the boundary condition for Bloch-Floquet periodicity at the edges of the chains with stress free boundaries makes **A** and **S** tri-diagonal matrices. The specific rules governing the nonzero elements of **A**, **S**, and **C** are detailed below [see Equations from (S4.9) to (S4.11)].

$$A_{k,l} = \begin{cases} k_1 + k_2 & \text{if} \quad k = l \\ -\left(k_1 \cdot \dfrac{1-(-1)^k}{2} + k_2 \cdot \dfrac{1+(-1)^k}{2}\right) & \text{if} \quad k = l \pm 1 \end{cases} \quad \text{(S4.9)}$$

$$S_{k,l} = \begin{cases} k_3 + k_4 & \text{if} \quad k = l \\ -\left(k_3 \cdot \dfrac{1-(-1)^k}{2} + k_4 \cdot \dfrac{1+(-1)^k}{2}\right) & \text{if} \quad k = l \pm 1 \end{cases} \quad \text{(S4.10)}$$

$$C_{k,l} = \{ s \quad \text{if} \quad k = l \quad \text{(S4.11)}$$

For the topological structure (Figure S4c), **M**, **K**, and **x** have dimensions of $2y \times 2y$, $2y \times 2y$, and $2y \times 1$, respectively. Introducing the topological interface modifies the rules of **A** and **S,** as shown in Equations (S4.12) and (S4.13).

$$A_{k,l} = \begin{cases} k_1 + k_2 & \text{if} \quad k = l \neq \dfrac{y+1}{2} \\ 2k_1 & \text{if} \quad k = l = \dfrac{y+1}{2} \\ -\left(k_1 \cdot \dfrac{1-(-1)^k}{2} + k_2 \cdot \dfrac{1+(-1)^k}{2}\right) & \text{if} \quad k = l \pm 1 < \dfrac{y+1}{2} \\ -\left(k_1 \cdot \dfrac{1+(-1)^k}{2} + k_2 \cdot \dfrac{1-(-1)^k}{2}\right) & \text{if} \quad k = l \pm 1 \geq \dfrac{y+1}{2} \end{cases} \tag{S4.12}$$

$$S_{k,l} = \begin{cases} k_3 + k_4 & \text{if} \quad k = l \neq \dfrac{y+1}{2} \\ 2k_3 & \text{if} \quad k = l = \dfrac{y+1}{2} \\ -\left(k_3 \cdot \dfrac{1-(-1)^k}{2} + k_4 \cdot \dfrac{1+(-1)^k}{2}\right) & \text{if} \quad k = l \pm 1 < \dfrac{y+1}{2} \\ -\left(k_3 \cdot \dfrac{1+(-1)^k}{2} + k_4 \cdot \dfrac{1-(-1)^k}{2}\right) & \text{if} \quad k = l \pm 1 \geq \dfrac{y+1}{2} \end{cases} \tag{S4.13}$$

### S4.2. Modal Compliance

The modal compliance analysis was performed for all the structures considered in the 1-D mass-spring models and presented in Figure 3a of the main manuscript. This analysis requires extraction of the effective mass ($m_{eff}$) and the angular resonance frequency ($\omega_{res}$) of each structure. This section describes our methodology for the extraction of these quantities.

The total kinetic energy ($KE_{tot}$) and the maximum particle velocity ($v_{\max}$) of each structure were extracted from the eigenvalues and mass-normalized eigenvectors obtained numerically by solving Equation (S4.1) in MATLAB. Then, the effective mass of each structure was calculated from its $v_{\max}$ as (S4.14) [1]:

$$m_{eff} = 2\frac{KE_{tot}}{v_{\max}^2} \tag{S4.14}$$

The extracted $m_{eff}$ and the corresponding $\omega_{res}$ value retrieved from the eigenvalue simulations were then used in Equation (1) of the main manuscript to calculate the modal compliance. Please note that the same approach was also used in the finite element methods (FEM) simulations used to extract the $C_{modal}$ values reported in Figure 4c of the main manuscript.

### S4.3. Dynamic Local Compliance

Similarly, our dynamic local compliance analysis was performed for the structures considered in our analytical study and presented in Figures 3b–3f of the main manuscript. This section describes the procedure used to calculate the dynamic local compliance.

After retrieving eigenvalues and eigenvectors of each structure (Equation (S4.1)), the frequency response of each system is calculated using modal superposition, as shown in Equation (S4.15).

$$\mathbf{x}(\omega_d) = \sum_{k=1}^{N} \frac{\boldsymbol{\phi}_k \cdot \boldsymbol{\phi}_k^T \cdot \mathbf{F}}{\omega_k^2 - \omega_d^2 + j\omega_k \omega_d \eta} \tag{S4.15}$$

where $N$ is the total number of masses in the corresponding structure; $\omega_k$ and $\boldsymbol{\phi}_k$ are eigenvalues and mass normalized eigenvectors of the system, respectively; **F** is the force; $\omega_d$ is the excitation angular frequency, and $\eta$ is the damping ratio that can be approximated as $1/Q$ for lightly damped systems. Finally, assuming a unit local force on each mass, dynamic local dynamic compliance is calculated as shown in Equation (S4.16).

$$\mathbf{C}_{\mathbf{Local}}(\omega_d) = \sum_{k=1}^{N} \frac{\left|\boldsymbol{\phi}_k\right|^2}{\omega_k^2 - \omega_d^2 + j\omega_k \omega_d \eta} \tag{S4.16}$$

[1] Piazza G, Stephanou PJ, Pisano AP. Piezoelectric Aluminum Nitride Vibrating Contour-Mode MEMS Resonators. Journal of Microelectromechanical Systems. 2006 Dec;15(6):1406–18.

## S5. Extraction of the Dispersion Curves and Zak Phase using Finite Element Modeling

### S5.1. Dispersion Curves

The dispersion curves of four different unit cell structures, namely, $UC_1$, $UC_2$, $UC_1^u$, $UC_2^u$, and the supercell of the topological structure were simulated using a commercial FEM tool. The schematics of the simulated cell structures are given in Figure S5a. The simulations were performed using the geometric parameter values listed in Table S1. In these simulations, Bloch-Floquet boundary conditions were assumed at the lateral edges of the corresponding cell structure with a periodicity of κ, where κ is the lateral wavevector. Then we swept κ across the first Brillouin zone and performed eigenfrequency study for each swept value of κ. The resulting dispersion curves presented in Figure 4a of the main manuscript show that while $UC_1$ and $UC_2$ possess a band gap, no such band exists for $UC_1^u$ and $UC_2^u$. Moreover, the resulting supercell dispersion curves confirm the existence of interface states inside the band gap of $UC_1$ and $UC_2$.

### S5.2. Zak Phases

Although $UC_1$ and $UC_2$ have the same dispersion curves, they have different Zak phases, which is the key factor leading to emergence of interface states in the proposed device. The Zak phases of these unit cells can be extracted by examining the parity of the mode shapes at the beginning and end of their dispersion branches [1]. This analysis was performed for the dispersion branches of $UC_1$ and $UC_2$ around the band gap. The dispersion curves of these unit cells are given in Figure S5b, along with the parities (Ps) of the mode shapes (+ for even mode, - for odd mode) at the beginning (κ=0) and end (κ=1) of their lower (green dots) and upper (blue dots) dispersion branches around the band gap. Based on these parity relations, the Zak phases ($\theta_{zak}$) of the lower and upper dispersion branches of $UC_1$ and $UC_2$ are reported in the same figure, showing that these unit cells possess opposite Zak phases. The mode shapes and their corresponding Ps used in this analysis are reported in Figure S5c.

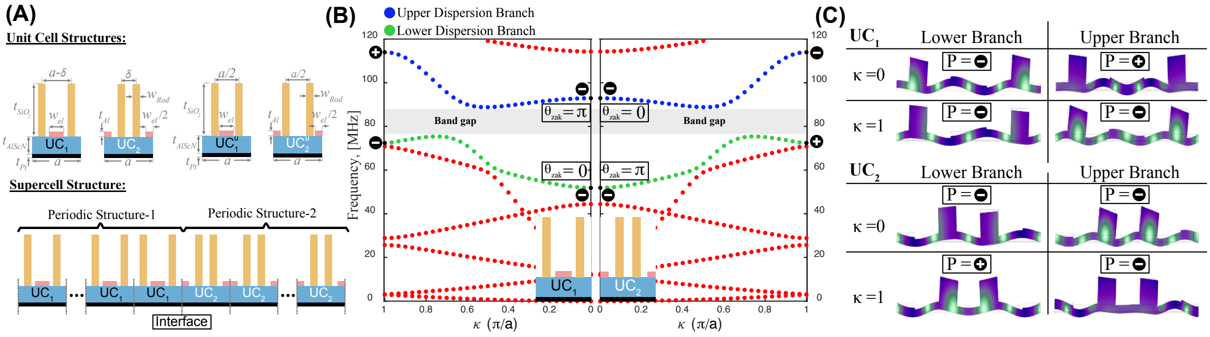


Figure S5: Dispersion analysis using finite element modeling : (a) Unit cell and supercell structures used in FEM dispersion analysis; (b) Dispersion curves of $UC_1$ and $UC_2$, including their parities at the start and end of the lower and upper dispersion branches around the band gap, and corresponding Zak phases; (c) Mode shapes of $UC_1$ and $UC_2$ at the start and end of lower and upper dispersion branches around the band gap.


[1] V. Gupta and B. Bradlyn, "Wannier-function methods for topological modes in one-dimensional photonic crystals," *Phys. Rev. A*, vol. 105, no. 5, p. 053521, May 2022, doi: 10.1103/PhysRevA.105.053521.

## S6. Velocity performance analysis of Rayleigh waves

We calculated $C_{modal}$ of Rayleigh waves using FEM by considering a Pt/AlScN slab on a 500 µm-thick silicon layer, named as the Rayleigh structure, as shown in Figure S6a. The Rayleigh structure assumes the same layer thicknesses as listed in Table S1. However, the slab length ($l$=1.72 µm) was adjusted such that the total mass of the Rayleigh structure matched that of devices analyzed in Figures 4b and 4c of the main manuscript. The out-of-plane displacement mode shape of the first Rayleigh mode of the Rayleigh structure is presented in Figure S6b, and its corresponding $C_{modal}$ was normalized with respect to that of IS-1 and is reported in Table S6, together with the normalized $C_{modal}$ values of the ISs. The results show that the ISs have up to 71x higher $C_{modal}$ than the Rayleigh mode that can be generated in a piezoelectric slab of equivalent mass.

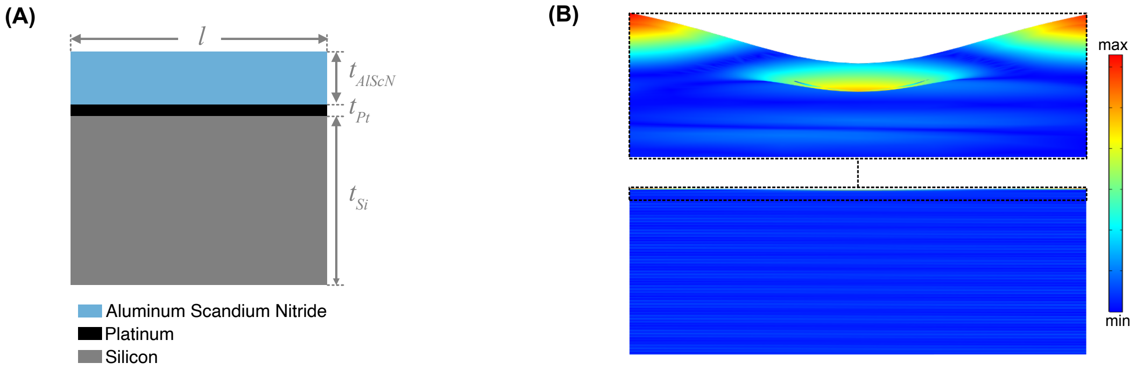


Figure S6: Velocity performance analysis of Rayleigh waves: (a) The Rayleigh structure used in the $C_{modal}$ FEM analysis; (b) The corresponding out-of-plane displacement mode shape of the Rayleigh mode of the Rayleigh structure

**Table S6 $C_{modal}$ values of the Rayleigh Mode and ISs normalized to that of IS-1**

| Mode | $C_{modal}$ |
|---|---|
| IS-1 | 1 |
| IS-2 | 0.48 |
| Rayleigh | 0.014 |

## S7. Comparison of Defect Modes with Topologically Protected Interface States

As discussed in the main manuscript, localized states can also be created using structural defects. Therefore, it is important to evaluate the advantages of topologically protected ISs transduced by the reported device over defect modes. This section compares the performance and robustness of topologically protected interface states and defect modes to local temperature changes. To ensure a fair comparison, a defect-mode device with similar fabrication complexity was designed using the periodic structure-1 employed in the topological device. Both devices have an identical number of unit cells, and the defect is introduced by removing a rod, as illustrated in Figure S7a. The temperature distributions of each device were simulated assuming a boundary heat source at the input terminal (Figure S7b). The resulting temperature distributions were scaled to represent local temperature changes (ΔT) ranging from 0 °C to 500 °C. Finally, the scaled temperature distributions were used to modify the elastic moduli of the forming materials according to their respective temperature coefficients of elastic modulus (TCEs), and the maximum out-of-plane particle velocities were extracted for each structure from frequency domain simulations for the same input drive voltage. The extracted out-of-plane particle velocities were normalized with respect to that of the IS-1 at ΔT=0 and are presented in Figure S7c. When there is no temperature change, the defect mode has ~10% lower out-of-plane particle velocity compared to IS-1. More importantly, for elevated temperatures the velocity of the defect mode significantly degrades, whereas IS-1 maintains its velocity performance thanks to the topological protection. Such thermal resilience of ISs permits to reach the maximum achievable particle velocity before nonlinearities or catastrophic failures occur by increasing the driving power. Without such thermal resilience, in fact, increasing the power does not necessarily lead to higher particle velocities, as shown for defect modes in Figure S7c below.

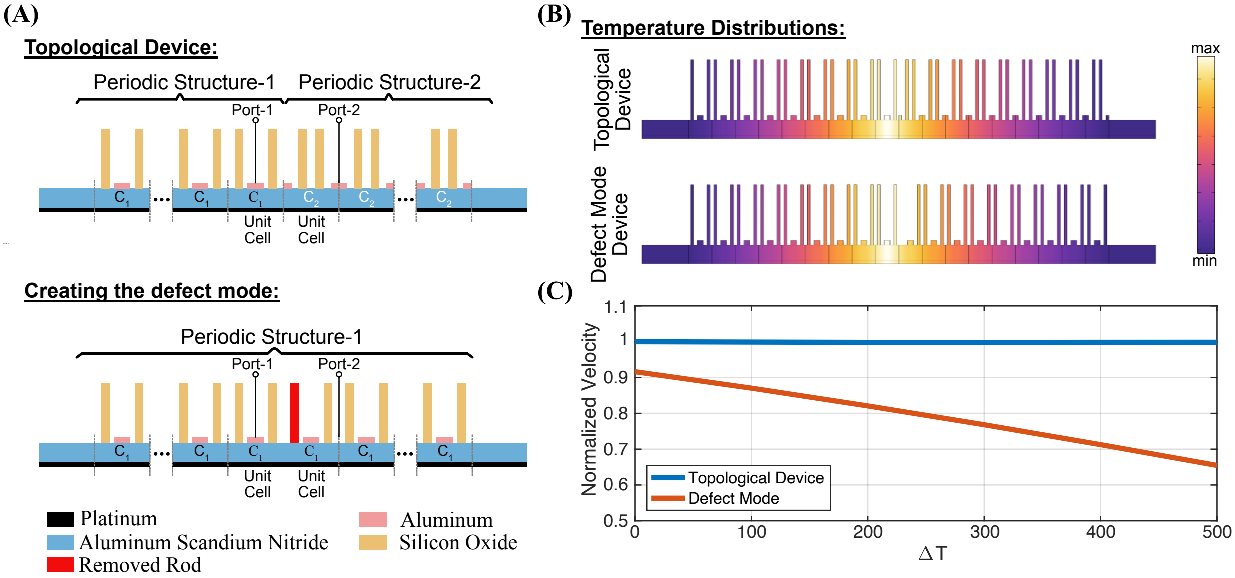


Figure S7: Comparison of velocity performance of the topological and defect mode devices: (a) The defect mode device is based on Periodic Structure-1, which has the same number of unit cells as the topological device but includes one missing rod to create the defect; (b) Simulated temperature distributions of both devices under a boundary heat source applied at Port-1; (c) Out-of-plane particle velocities of both devices, normalized to that of the topological device at ΔT=0, showing that the topological device has a higher and more robust out-of-plane velocity against local temperature variations compared to the defect mode device.

## S8. Fabrication

The device was fabricated on a high-resistivity silicon substrate. The process began with the sputtering of a 100 nm-thick platinum (Pt) layer, followed by the reactive co-sputtering of a 500 nm-thick aluminum scandium nitride (AlScN) layer in the same deposition chamber, without breaking vacuum. Next, a silicon oxide ($SiO_2$) hard mask was deposited via plasma-enhanced chemical vapor deposition (PECVD) and patterned using reactive ion etching (RIE). This hard mask defined the release windows. Subsequently, the AlScN and Pt layers were etched through inductively coupled plasma reactive ion etching (ICP-RIE). After patterning, the $SiO_2$ hard mask was stripped using hydrofluoric acid (HF). Following that, a 2 µm-thick $SiO_2$ layer was deposited by PECVD. This oxide layer was patterned by RIE in two steps: first to form the rods of the periodic structures, targeting near-vertical sidewalls, and then to define islands for the routing traces and signal pads, intentionally achieving ~45˚ edge profiles. These $SiO_2$ islands serve to reduce the undesired capacitance between the probing pads and the bottom electrode, while the ~45˚ sidewalls help minimize the additional resistance introduced as the metal traces ascend onto these islands. Then, a 150 nm-thick aluminum layer was sputtered and patterned by liftoff to form the electrodes and routing traces. Subsequently, a 200 nm gold was evaporated to create the probing pads. Finally, the silicon underneath the device was removed by xenon difluoride ($XeF_2$) vapor-phase etching through the release windows, resulting in a fully suspended device structure. A process flow chart summarizing the fabrication process is presented in Figure S8.

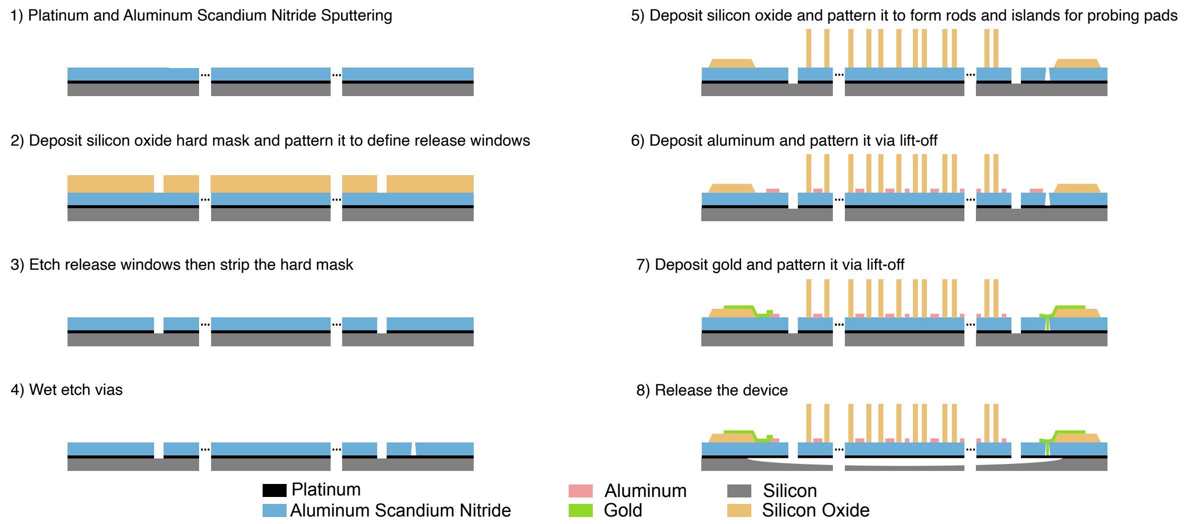


Figure S8: Process flow chart of the fabricated topological device

## S9. Experimental Verification for the Existence of Interface States

The fabricated device was wire-bonded to a printed circuit board (PCB). Firstly, its electrical response was characterized through a two-port scattering parameter measurement using a vector network analyzer. The measured $S_{21}$ response is given in Figure S9a, showing two peaks corresponding to IS-1 and IS-2. Following that, the out-of-plane displacement distributions around the interface for both ISs were measured using a laser Doppler vibrometer (LDV) and presented in Figure S9b. Consistent with our predictions from the toy model and finite element simulations, IS-1 exhibits a higher out-of-plane displacements compared to IS-2.

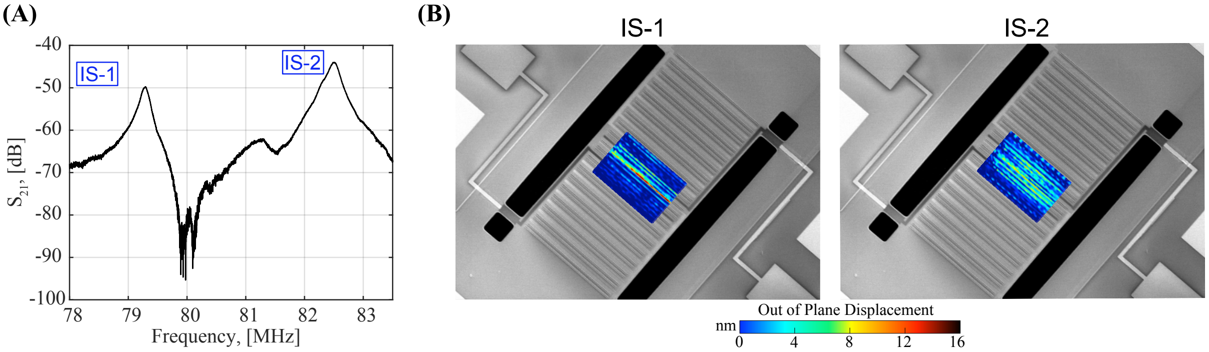


Figure S9: Electrical and laser Doppler vibrometer measurements of the topological device: (a) Two-port scattering parameter measurements; (b) Out-of-plane displacement distributions of IS-1 and IS-2 around the interface.

## S10. Absorbed Power Estimation

To better evaluate the effect of nonlinearities, we analyzed the velocity performance of the device under test (DUT) considering the power absorbed by it. Estimation of the absorbed power relies on the 2-Port scattering (S2P) response of the DUT. We imported this response to a commercial circuit simulator and run a harmonic balance simulation at the corresponding frequency, i.e., the frequency of the interface state-1 ($f_{IS-1}$). The schematic of the simulated circuit is shown in Figure S10, which employs current probes at each port of the device estimating input power to device ($P_{in}$) and output power ($P_{out}$) from the device. The absorbed power ($P_{abs}$) was then estimated as shown in Equation (S10.1).

$$P_{abs} = P_{in} - P_{out} \tag{S10.1}$$

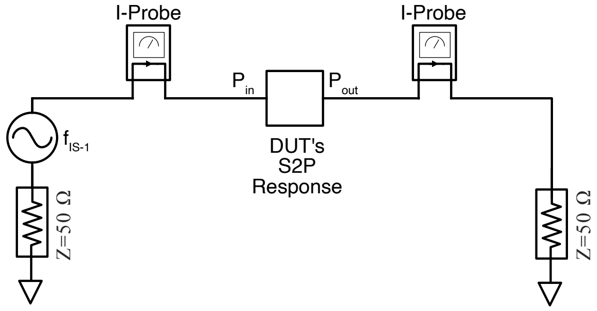


Figure S10: Schematic employed in the harmonic balance simulation to estimate the absorbed power.

## S11. Experimental Test Setup for High Drive Power Characterization

The displacement of the device under high drive power levels is characterized using a homodyne polarized Michelson interferometer [1], a vector network analyzer (VNA), and an RF power amplifier. The device was driven through a VNA and an RF power amplifier while its scattering parameters are simultaneously monitored. The interferometer setup uses a linearly polarized HeNe laser beam. An optical isolator is attached to the laser source to suppress back-reflections. Firstly, the polarization of the laser beam is rotated using a half-wave (λ/2) plate set at 22.5°, and equal p- and s- polarized components are created. Then a beam expander expands the laser beam to match the entrance pupil of the objective, and a polarizing beam splitter (PBS) separates the beam into the reference arm (reflected) and to the sensing arm (transmitted). Each arm has a quarter-wave (λ/4) plate that converts linear polarization into circular. The sense arm focuses the beam onto the device under test, in particular, to the interface of the topological device, through the objective. On the other hand, the beam on the reference arm is reflected from a piezoelectrically actuated movable mirror. The reflected beams from both sense and reference arms pass back through their corresponding λ/4 plates and are converted back to linear-but orthogonal orientation, allowing recombination of two beams at the PBS. The combined beam's polarization states are rotated using a λ/4 plate to enable interference. The beam is then split into two arms using a non-polarizing beam splitter (BS). The transmitted beam passes through another PBS and is reflected onto photodiode-1 (PD-1). PD-1 provides the direct interferometric signal readout to a spectrum analyzer. The reflected arm from the BS goes through a λ/4 plate and polarizer, then focused on the photodiode-2 (PD-2), generating a quadrature signal with a π/2 phase shift relative to PD-1. PD-2's signal is used as feedback in a proportional-integral-derivative (PID) controller to set the position of the movable mirror for optimal interference.

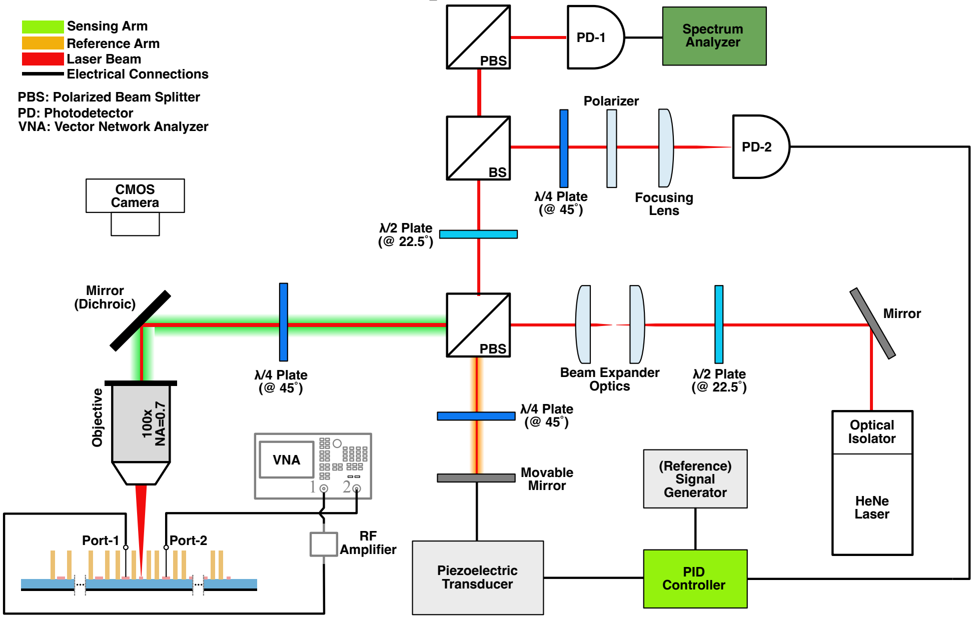


Figure S11: Interferometric displacement characterization setup for higher RF powers.

[1] V. Bello, A. B. Ari, M. Selim Hanay and K. L. Ekinci, "Measurement and Characterization of Nano-Electro-Mechanical Systems Using Laser Interferometry," 2020 IEEE International Instrumentation and Measurement Technology Conference (I2MTC), Dubrovnik, Croatia, 2020, pp. 1-5, doi: 10.1109/I2MTC43012.2020.9129282.

## S12. FEM Out-of-Plane Displacement Amplitude the First Principal Stress

The main manuscript reports a straight crack located near the common interface of Periodic Structure-1 and Periodic Structure-2. The crack location corresponds to the region with maximum out-of-plane displacement and maximum principal stress in our FEM simulations, as depicted in Figure S12.

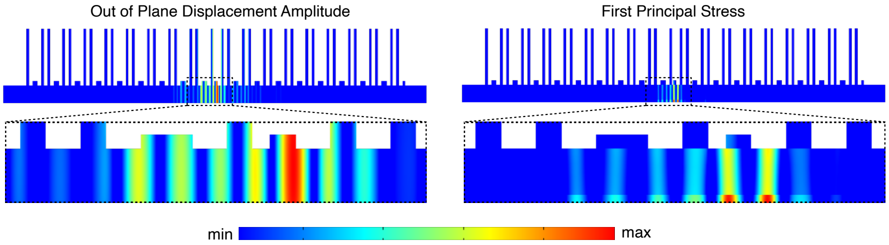


Figure S12: Simulated out-of-plane displacement amplitude and first principal stress distributions, showing that the location of the failure coincides with the region of maximum out-of-plane displacement and first principal stress.

## S13. Trivial Device

We studied the differences between the performance achievable by IS-1 and those attained by trivial modes, as presented in Figure 5g of the main manuscript. Unlike IS-1, trivial modes are not localized. Therefore, for the comparable degrees of nonlinearity, IS-1 achieves almost 4 times higher maximum particle velocity than that of the trivial mode. For this comparison, we used a trivial device fabricated on the same chip as the reported topological device. This section compares the trivial device design with that of the topological device and reports their $S_{21}$ measurements.

Figure S13a compares the designs of the topological and trivial devices. Both devices consist of a total of 18 unit cells and they have the same geometric dimensions as listed in Table S1. However, the trivial device consists of only $UC_1$; therefore, unlike the topological device, it doesn't have an interface with broken periodicity. $S_{21}$ measurements of these devices are reported in Figure S13b. The topological device exhibits a resonance frequency at 79.3 MHz with a $Q_{3\text{-dB}}$ of 477, while the trivial device has a resonance frequency of 74.3 with a $Q_{3\text{-dB}}$ of 334.

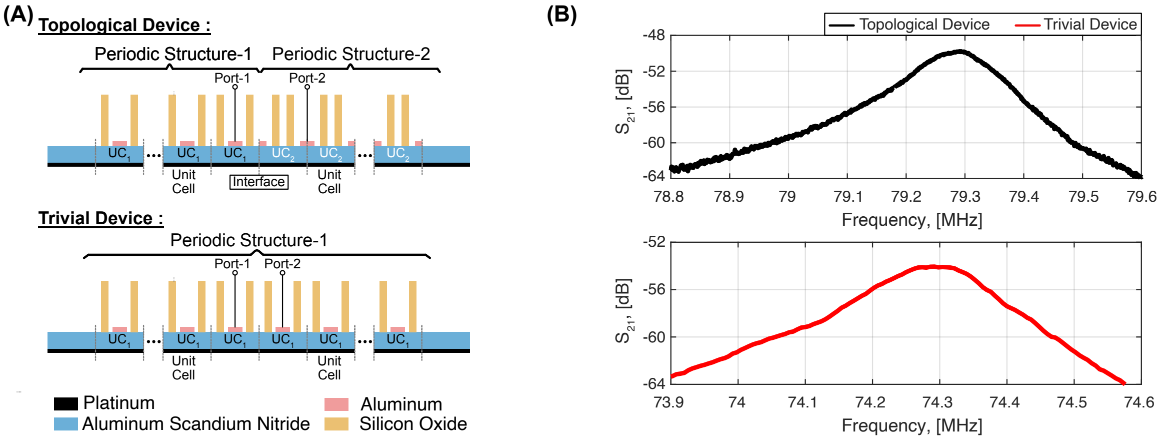


Figure S13: Comparison of the topological and trivial device: (a) Design comparison showing that the topological device consists of two different unit cells forming an interface between two periodic structures, while the trivial device is formed by a chain of only one type of unit cell; (b) $S_{21}$ responses of the topological and trivial devices.

## S14. Prospects of Using Localized States in Inertial Sensing

A gyroscope with matched drive and sense modes operating at an angular frequency $\omega_{op}$ and having a mass $m$ can be represented as shown in Figure S14 below.

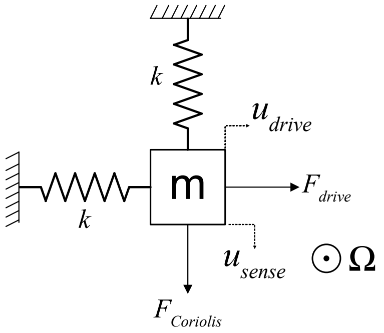


Figure S14: Schematic representation of a mode-matched gyroscope

When the gyroscope is driven by a force $F_{drive}$ at its operational frequency, the resulting displacement is given Equation (S14.1).

$$u_{drive} = \frac{F_{drive}}{k} Q_{drive} \tag{S14.1}$$

When the device is subjected to an external angular rate Ω, a Coriolis force is generated as shown in Equation (S14.2).

$$F_{Coriolis} = 2m\Omega \dot{u}_{drive} = 2m\Omega\omega_{op} u_{drive} \tag{S14.2}$$

The displacement induced by the Coriolis force and the corresponding mechanical scale factor ($SF_{mech}$) of the gyroscope can be found as shown in Equations (S14.3) and (S14.4), respectively.

$$u_{sense} = \frac{F_{Coriolis}}{k} Q_{sense} = \frac{2m\Omega\omega_{op} u_{drive}}{k} Q_{sense} \tag{S14.3}$$

$$SF_{Mech} = \frac{u_{sense}}{\Omega} = \frac{2m\omega_{op} u_{drive}}{k} \tag{S14.4}$$

Finally using (S14.1) and (S14.4) we find that $SF_{mech}$ scales with $\sqrt{m}$ and $1/k\sqrt{k}$ as shown in Equation (S14.5).

$$SF_{Mech} \propto \frac{Q_{sense} Q_{drive}}{k} \sqrt{\frac{m}{k}} \tag{S14.5}$$

Equation (S14.5) reveals that for any targeted operational frequency, it is always preferred to have MEMS gyroscopes with lower modal stiffness (i.e., larger modal compliance) to achieve a higher scale factor. At the same time, higher frequency operation is desired for wide bandwidth and high resilience to shock and vibration. However, operating at higher frequencies typically comes with a larger $k$, which reduces $SF_{mech}$.

The proposed topological device in this study allows high-frequency operation with a significantly lower $k$ than possible when exploiting traditional SAW/BAW modes. Therefore, it has the potential to achieve MEMS gyroscopes with both a superior scale factor and high resilience to shock and vibration.
